# Supplementary material for: SERPENT-VLM : Self-Refining Radiology Report Generation Using Vision Language Models
Source: arXiv:2404.17912 source file (2024-07-18)
Supplement: Supplementary file 1 [file supplementary_material.tex]

\section{Supplementary Material}
\label{Chapter_supplementary}
\noindent\textbf{Robustness to Noisy Input Images} 

An essential aspect of our experimental evaluation was to determine the robustness of radiology report generation models to real-life image quality, which can often be low and noisy. To this end, we conducted experiments where Gaussian noise was added to radiological images before they were fed into the visual encoder. This approach aimed to simulate the varying quality of real-life medical images and assess the resilience of the models in generating accurate and comprehensive radiological reports under such conditions. We compared the performance of SERPENT-VLM, our proposed model, with two other models: LlaVA-Med \cite{li2023llavamed}, a current state-of-the-art generalistic medical model based on LLaMA-2, and BiomedGPT \cite{zhang2024biomedgpt}, a generalistic medical domain pre-trained GPT-based model.

\begin{figure}[H]
\centering
\includegraphics[width=0.8\textwidth]{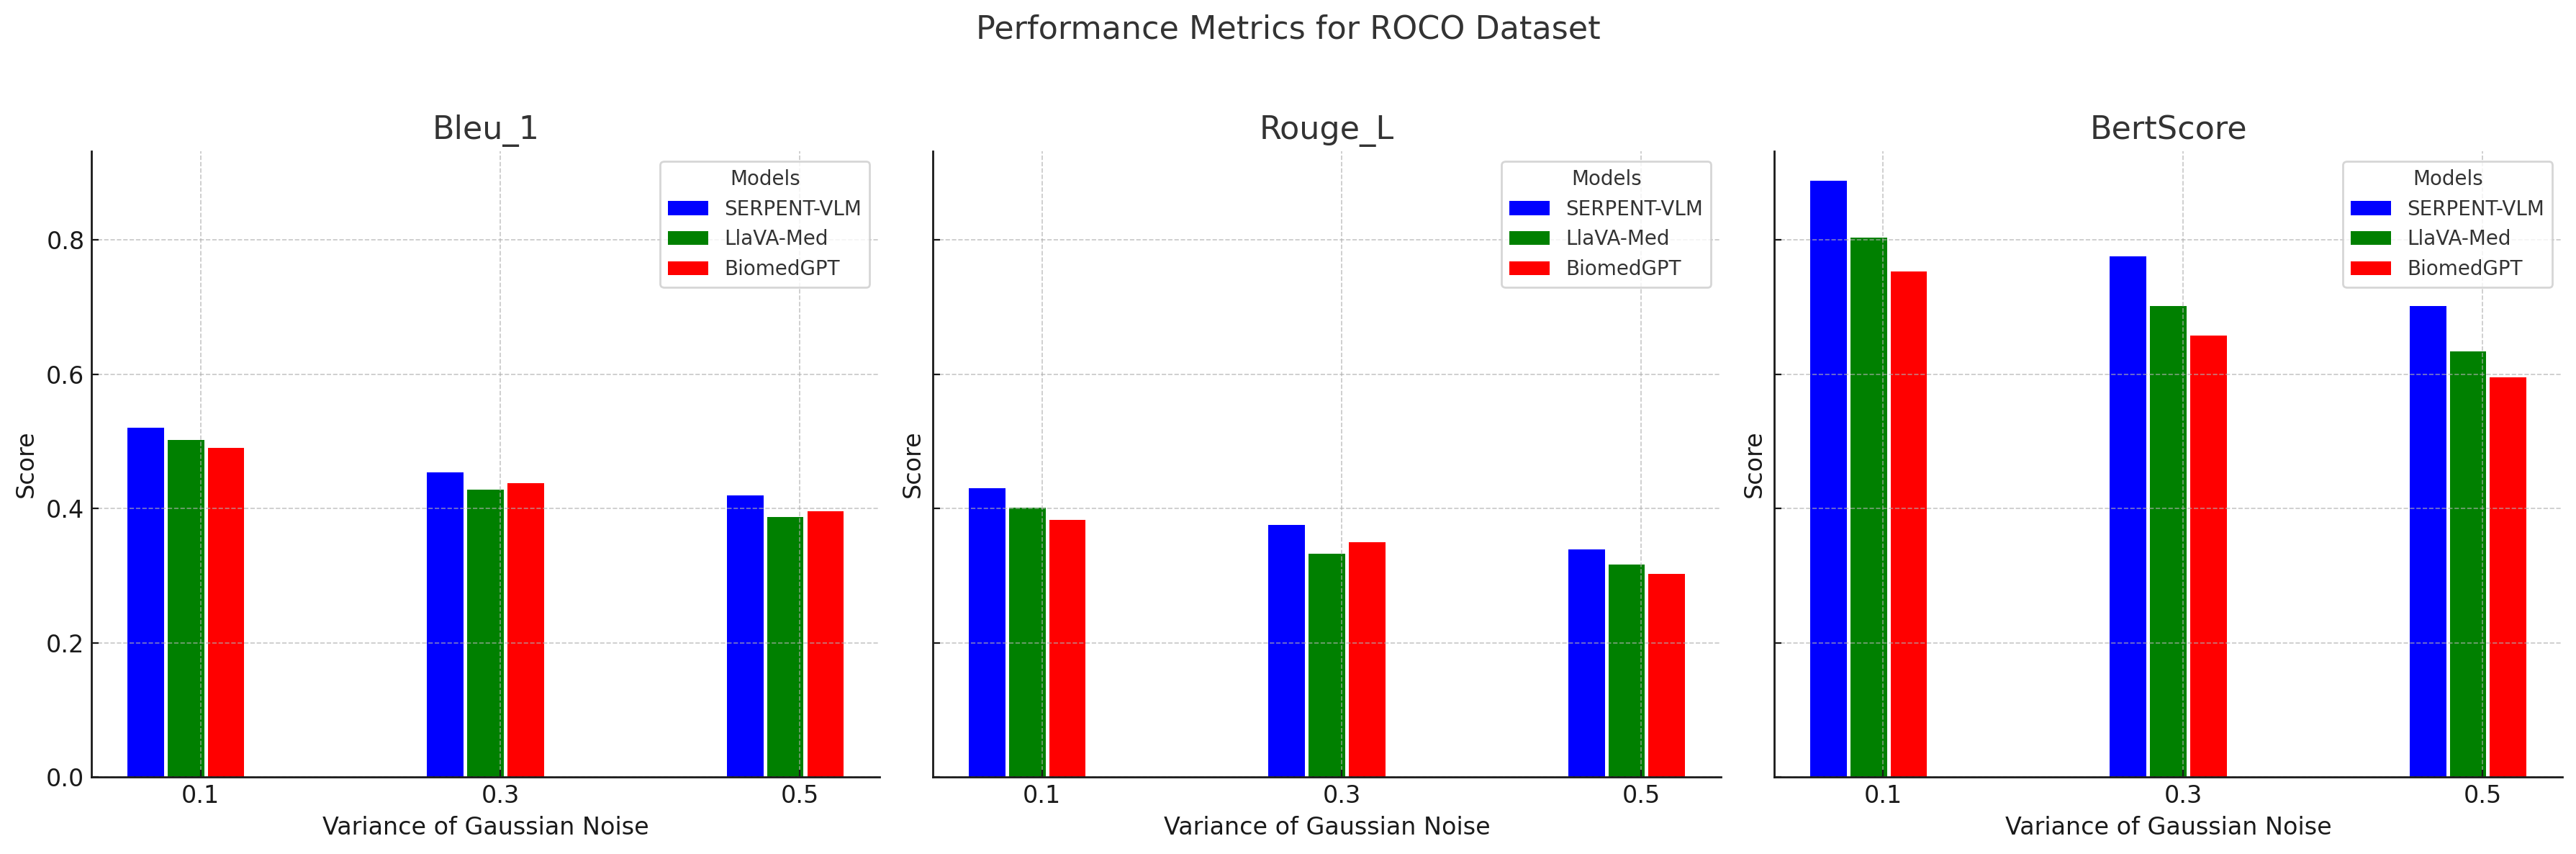}
\caption{Performance metrics for ROCO dataset with varying levels of Gaussian noise.}
\label{fig:roco_noise}
\end{figure}

\begin{figure}[H]
\centering
\includegraphics[width=0.8\textwidth]{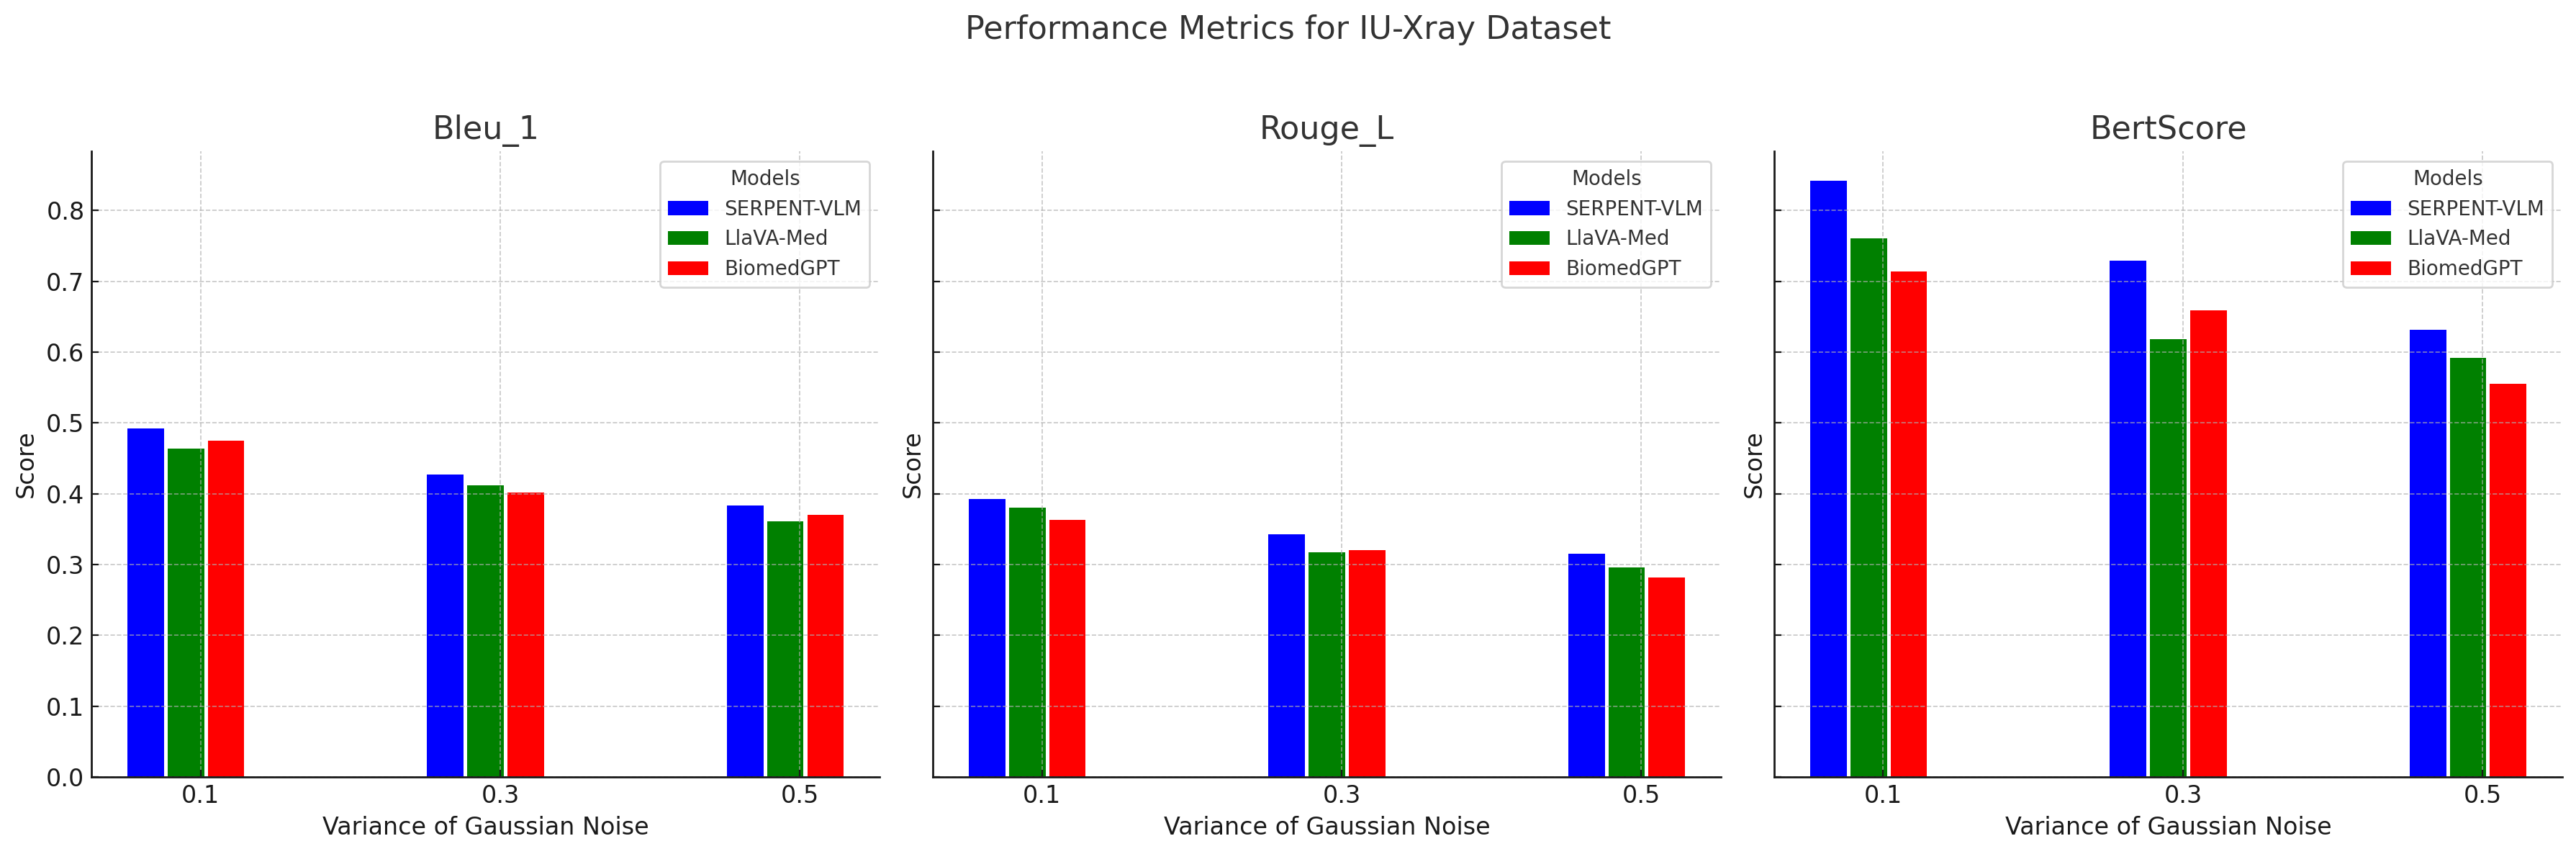}
\caption{Performance metrics for IU-Xray dataset with varying levels of Gaussian noise.}
\label{fig:iuxray_noise}
\end{figure}

Observations from Figures \ref{fig:roco_noise} and \ref{fig:iuxray_noise} demonstrate the superior robustness and resilience of SERPENT-VLM to noisy inputs compared to LlaVA-Med and BiomedGPT. Notably, SERPENT-VLM consistently outperforms the other models across all levels of Gaussian noise variance for both datasets. For instance, in the presence of moderate noise (variance of 0.3), SERPENT-VLM maintains a higher $BLEU_1$ score, indicating its capacity to preserve the coherence and relevance of the generated reports even under degraded input conditions. This trend is consistent across other performance metrics, including $Rouge_L$ and $BertScore$, underscoring SERPENT-VLM's superior ability to extract and utilize relevant information from noisy images effectively.

Furthermore, the decline in performance metrics is less pronounced for SERPENT-VLM as the noise level increases, compared to the other models. This indicates not only the model's resilience but also its potential applicability in clinical settings, where image quality can significantly vary. Such robustness to noise is crucial for deploying automated radiology report generation systems in real-world medical settings, where they can support radiologists by providing reliable, accurate, and timely reports even when the image quality is suboptimal.

These experiments highlight the advanced capability of SERPENT-VLM in handling real-life challenges of radiological image quality, making it a promising tool for enhancing diagnostic efficiency and accuracy in the medical domain.
